# Supplementary material for: Efficient implementation of molecular CCSD gradients with Cholesky-decomposed electron repulsion integrals
Source: arXiv:2202.02019 source file (2022-02-04)
Supplement: Supplementary file 1 [file SI.pdf]

# Efficient implementation of molecular CCSD gradients with Cholesky-decomposed electron repulsion integrals

Anna Kristina Schnack-Petersen,[1] Henrik Koch,[2,3] Sonia Coriani,[1,3] and Eirik F. Kjønstad[3,a)]

[1)] *Department of Chemistry, Technical University of Denmark, 2800 Kongens Lyngby, Denmark*

[2)] *Scuola Normale Superiore, Piazza dei Cavaleri 7, 56126 Pisa, Italy*

[3)] *Department of Chemistry, Norwegian University of Science and Technology, 7491 Trondheim, Norway*

(Dated: 3 February 2022)

[a)] Electronic mail: eirik.kjonstad@ntnu.no

## I. COMPARISONS OF CALCULATION TIMES WITH AND WITHOUT FROZEN CORE APPROXIMATION IN Q-CHEM

| | frozen core† | | | non-frozen core | | |
|---|---|---|---|---|---|---|
| | Cycles | Time | $\frac{\text{Time}}{\text{Cycle}}$ | Cycles | Time | $\frac{\text{Time}}{\text{Cycle}}$ |
| Thymine (GS) | 9 | 3 h 45 m | 25 m | 10 | 6 h 22 m | 38 m |
| Thymine (ES) | 6 | 3 h 40 m | 37 m | 7 | 7 h 01 m | 1 h |
| Azobenzene (GS) | 7 | 16 h 33 m | 2 h 22 m | 7 | 1 d 2 h 08 m | 3 h 44 m |
| Azobenzene (ES) | 7 | 1 d 2 h 47 m | 3 h 50 m | 6 | 1d 13 h 40m | 6 h 17 m |

TABLE I. Comparisons of calculation time in Q-Chem with and without the frozen core approximation.

† The calculation was run with 800 GB memory available
